# Supplementary material for: MTBBench: A Multimodal Sequential Clinical Decision-Making Benchmark in Oncology
Source: arXiv:2511.20490 source file (2025-11-25)
Supplement: Supplementary file 1 [file appendix_examples.tex]

\begin{tcolorbox}[colback=blue!5!white, colframe=blue!75!black, title=Question, boxsep=1pt, left=2pt, right=2pt, top=2pt, bottom=2pt]
    What is the primary histologic type of the tumor according to the H\&E images?
A) Adenocarcinoma, non-keratinizing  
B) Squamous cell carcinoma, non-keratinizing  
C) Squamous cell carcinoma, keratinizing  
D) Small-cell neuroendocrine carcinoma  
E) Undifferentiated carcinoma  
F) Mucinous aden
    \end{tcolorbox}

    \begin{tcolorbox}[title=Example of InternVL3-38b on H\&E question, colframe=black!80!white, colback=white, boxsep=1pt, left=1pt, right=1pt, top=1pt, bottom=1pt]
    \begin{minipage}[t]{0.48\textwidth}
    
    \begin{tcolorbox}[title=No Tools Available, colback=red!5, boxsep=1pt, left=2pt, right=2pt, top=2pt, bottom=2pt]
    \begin{tcolorbox}[colback=gray!10, title=Conversation, boxsep=1pt, left=1pt, right=1pt, top=1pt, bottom=1pt]
\textbf{Assistant:} [REQUEST: PrimaryTumor\_HE\_104.jpg] [REQUEST: PrimaryTumor\_HE\_104\_roi.jpg] \\[1pt]
\textbf{User:} [2 FILES INCLUDED] was accessed by you
You can access all these files once again if necessary by asking for them in the format [REQUEST: filename.extension]. \\[1pt]
\textbf{Assistant:} Based on the provided H\&E images, the tumor exhibits a high density of small, round cells with scant cytoplasm and hyperchromatic nuclei, which are characteristic features of small-cell neuroendocrine carcinoma. The lack of keratinization and the presence of a high nuclear-to-cytoplasmic ratio further support this diagnosis. \\[1pt]
\end{tcolorbox}

    \textbf{Answer:} D) Small-cell neuroendocrine carcinoma

    \textbf{Files Accessed:}\\
    \begin{center}
\includegraphics[width=0.25\linewidth]{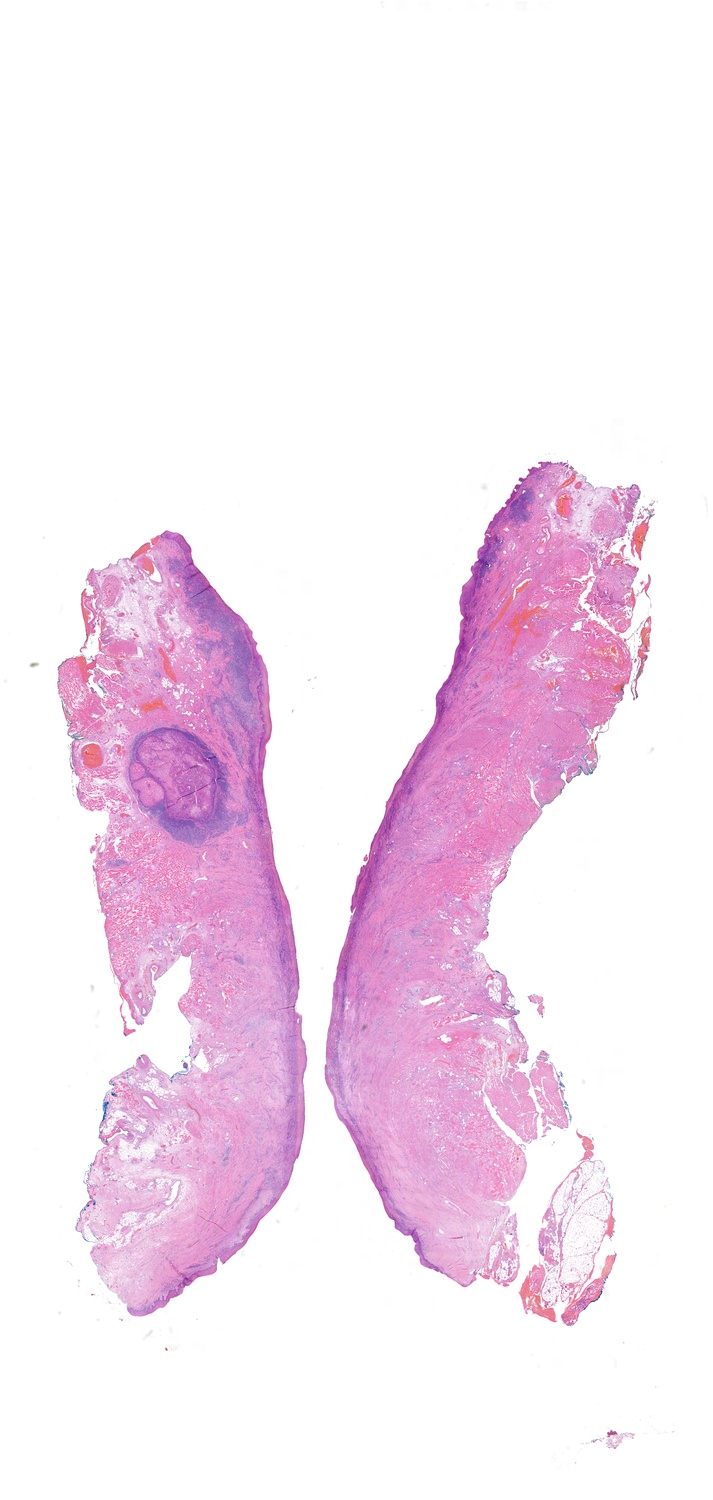}
\includegraphics[width=0.25\linewidth]{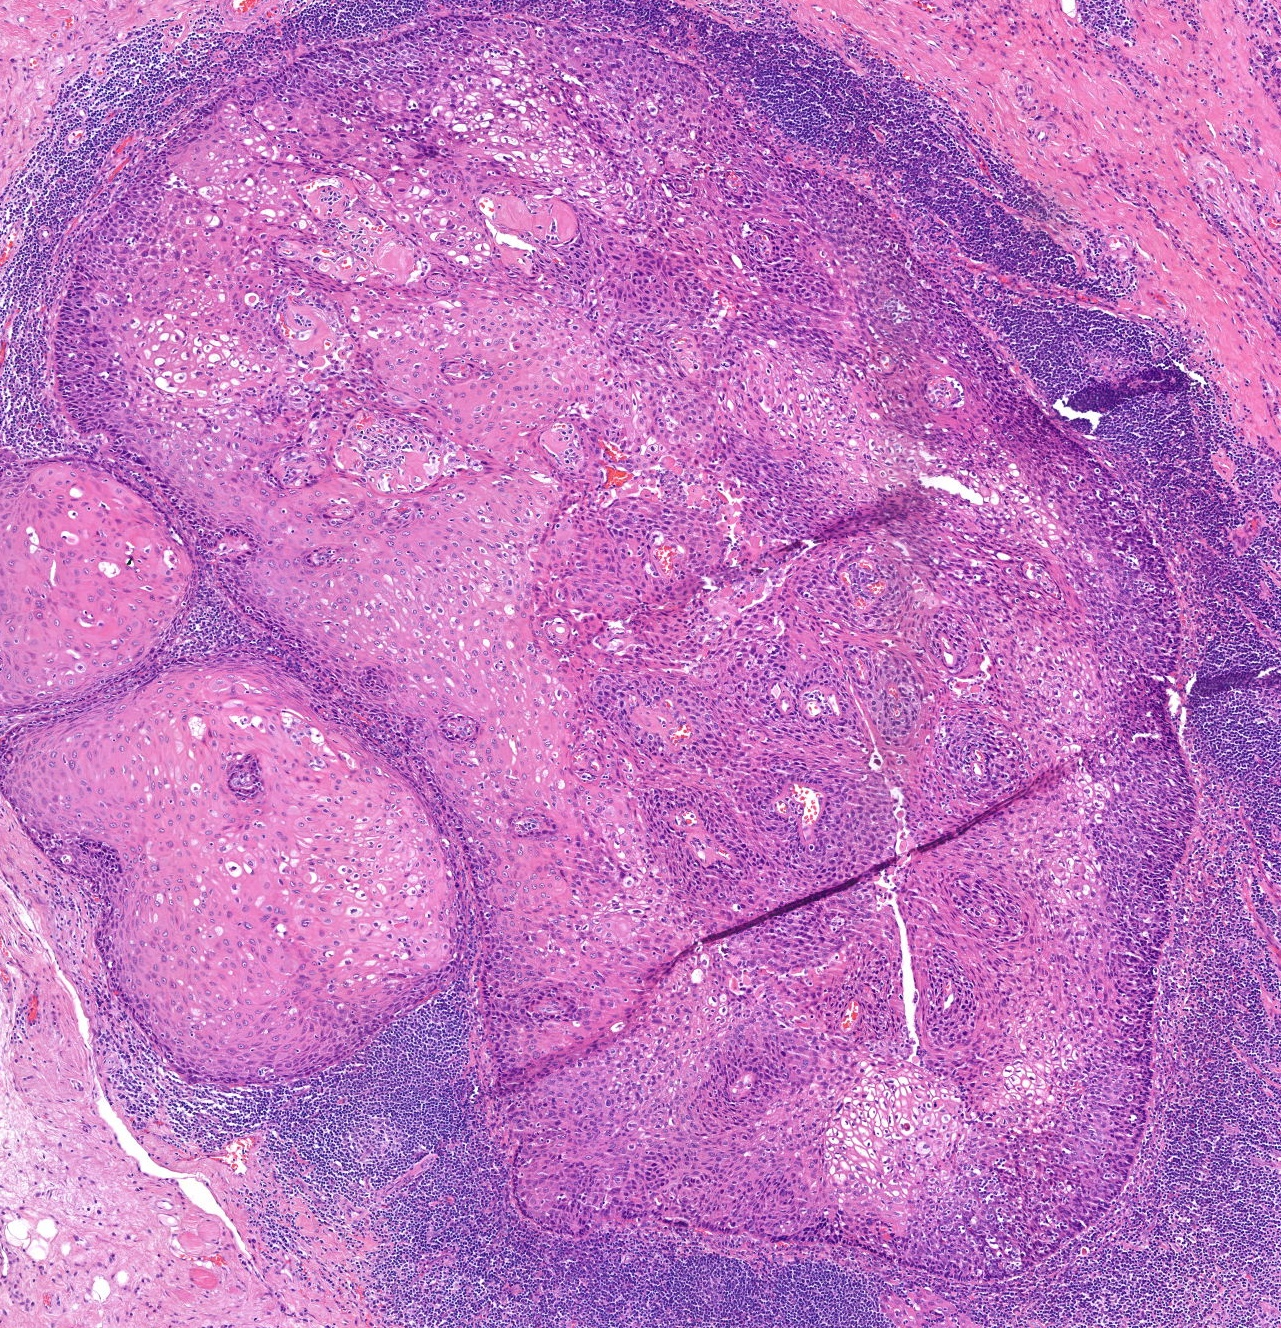}
\end{center}
\textit{}


    \textbf{Tools Used:} None
    \end{tcolorbox}
    \end{minipage}\hfill
    \begin{minipage}[t]{0.48\textwidth}
    \begin{tcolorbox}[title=Tools Available, colback=green!5, boxsep=1pt, left=2pt, right=2pt, top=2pt, bottom=2pt]
    \begin{tcolorbox}[colback=gray!10, title=Conversation, boxsep=1pt, left=1pt, right=1pt, top=1pt, bottom=1pt]
\textbf{Assistant:} [REQUEST: PrimaryTumor\_HE\_104.jpg] [REQUEST: PrimaryTumor\_HE\_104\_roi.jpg]

[CONCH: PrimaryTumor\_HE\_104.jpg, (Adenocarcinoma, non-keratinizing), (Squamous cell carcinoma, non-keratinizing), (Squamous cell carcinoma, keratinizing), (Small-cell neuroendocrine carcinoma), (Undifferentiated carcinoma), (Mucinous adenocarcinoma)] \\[1pt]
\textbf{User:} [2 FILES INCLUDED] included in your context\\[1pt]
\textbf{Assistant:} [CONCH: PrimaryTumor\_HE\_104.jpg, (Adenocarcinoma, non-keratinizing), (Squamous cell carcinoma, non-keratinizing), (Squamous cell carcinoma, keratinizing), (Small-cell neuroendocrine carcinoma), (Undifferentiated carcinoma), (Mucinous adenocarcinoma)]

[CONCH: PrimaryTumor\_HE\_104\_roi.jpg, (Adenocarcinoma, non-keratinizing), (Squamous cell carcinoma, non-keratinizing), (Squamous cell carcinoma, keratinizing), (Small-cell neuroendocrine carcinoma), (Undifferentiated carcinoma), (Mucinous adenocarcinoma)] \\[1pt]
\textbf{User:} The image resembles Squamous cell carcinoma, keratinizing with very high probability.
The image resembles Squamous cell carcinoma, keratinizing with medium probability.You can use this information, but keep in mind that CONCH is not perfect and you should also use your own reasoning. \\[1pt]
\textbf{Assistant:} Based on the CONCH model's assessment and the provided H\&E images, the primary histologic type of the tumor is most likely: \\[1pt]
\end{tcolorbox}

    \textbf{Answer:} C) Squamous cell carcinoma, keratinizing

    \textbf{Files Accessed:}\\
    \begin{center}
\includegraphics[width=0.25\linewidth]{example_case_figs/PrimaryTumor_HE_104.jpg}
\includegraphics[width=0.25\linewidth]{example_case_figs/PrimaryTumor_HE_104_roi.jpg}
\end{center}
\textit{}


    \textbf{Tools Used:} CONCH
    \end{tcolorbox}
    \end{minipage}
    \end{tcolorbox}








\begin{tcolorbox}[colback=blue!5!white, colframe=blue!75!black, title=Question, boxsep=1pt, left=2pt, right=2pt, top=2pt, bottom=2pt]
    Based on both H\&E and IHC images, what is the likely relationship between the observed perinodal invasion and immune cell infiltration at the InvasionFront?
A) High CD3+ and CD8+ T-cell infiltration likely prevents perinodal invasion  
B) High CD68+ macrophage infiltration at the InvasionFront may facilitate perinodal invasion  
C) Low CD56+ lymphocyte presence at the
    \end{tcolorbox}

    \begin{tcolorbox}[title=Example of InternVL3-38b on IHC question, colframe=black!80!white, colback=white, boxsep=1pt, left=1pt, right=1pt, top=1pt, bottom=1pt]
    \begin{minipage}[t]{0.48\textwidth}
    \begin{tcolorbox}[title=No Tools Available, colback=red!5, boxsep=1pt, left=2pt, right=2pt, top=2pt, bottom=2pt]
    \begin{tcolorbox}[colback=gray!10, title=Conversation, boxsep=1pt, left=1pt, right=1pt, top=1pt, bottom=1pt]
\textbf{Assistant:} [REQUEST: \textit{IHC at Invasion Front for all markers}]\\[1pt]
\textbf{User:} [12 FILES INCLUDED] was accessed by you
You can access all these files once again if necessary by asking for them in the format [REQUEST: filename.extension]. \\[1pt]
\textbf{Assistant:} Based on the provided IHC images, the likely relationship between the observed perinodal invasion and immune cell infiltration at the InvasionFront is:

B) High CD68+ macrophage infiltration at the InvasionFront may facilitate perinodal invasion

The images show significant CD68+ macrophage infiltration at the InvasionFront, which can contribute to the tumor's ability to invade and spread to lymph nodes by modulating the immune response and creating a conducive microenvironment for metastasis. \\[1pt]
\textbf{User:} Please provide the final answer in  specifying the answer choice letter you picked (A, B, C, D, E, or F) or ask for files with [REQUEST: filename.extension]. \\[1pt]
\textbf{Assistant:}  \\[1pt]
\end{tcolorbox}

    \textbf{Answer:} B) High CD68+ macrophage infiltration at the InvasionFront may facilitate perinodal invasion

    \textbf{Files Accessed:}\\
    \begin{center}
\includegraphics[width=0.25\linewidth]{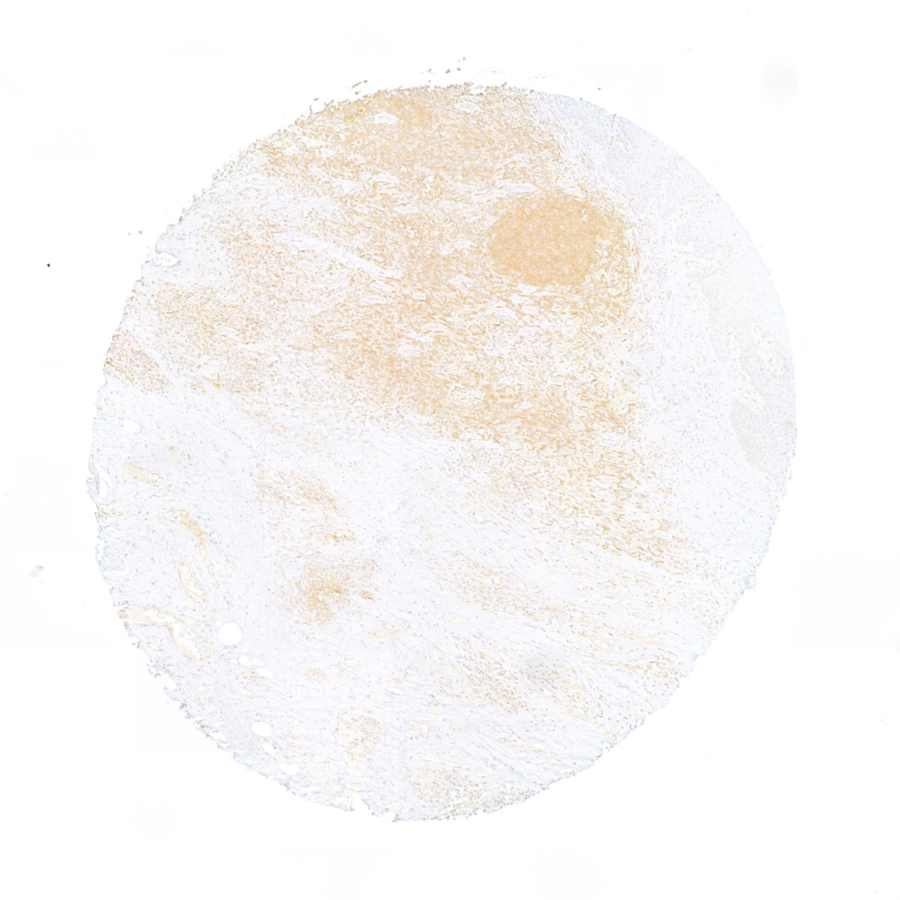}
\includegraphics[width=0.25\linewidth]{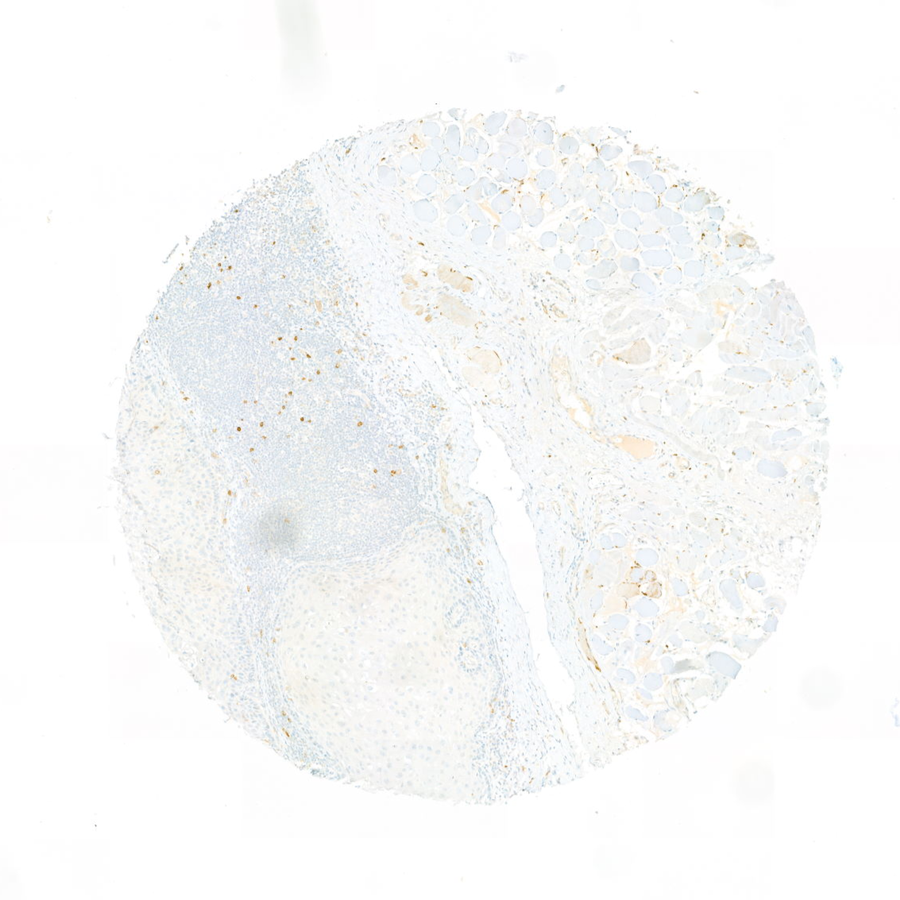}
\includegraphics[width=0.25\linewidth]{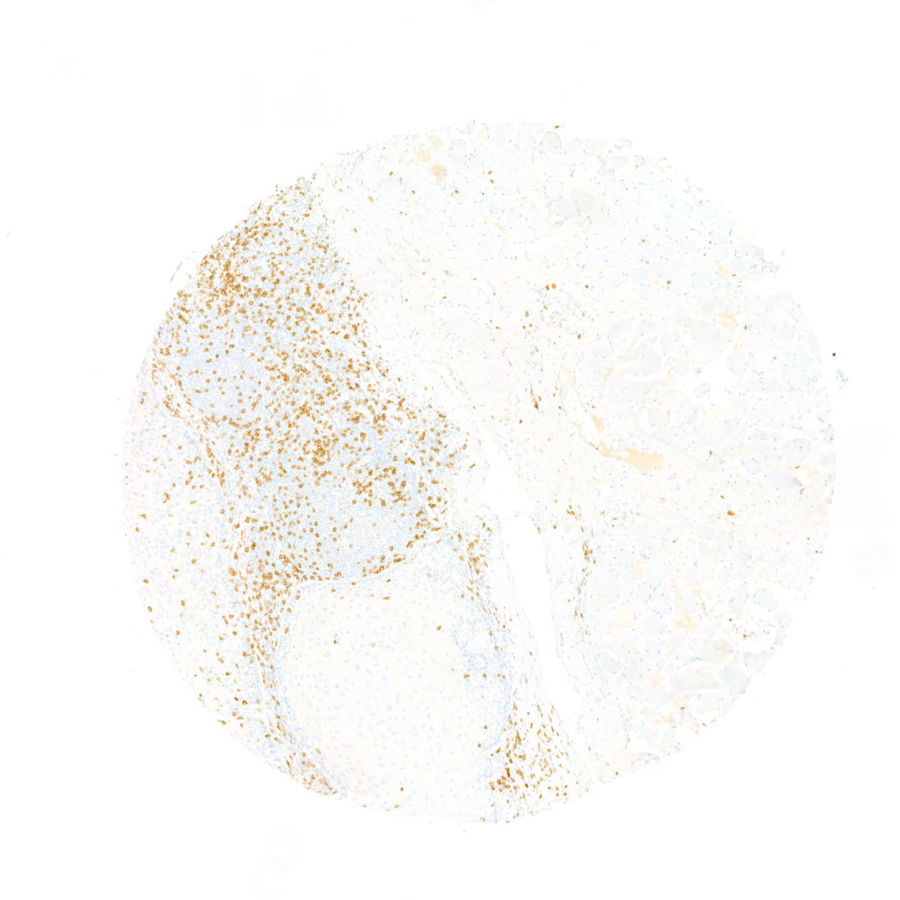}
\\
\includegraphics[width=0.25\linewidth]{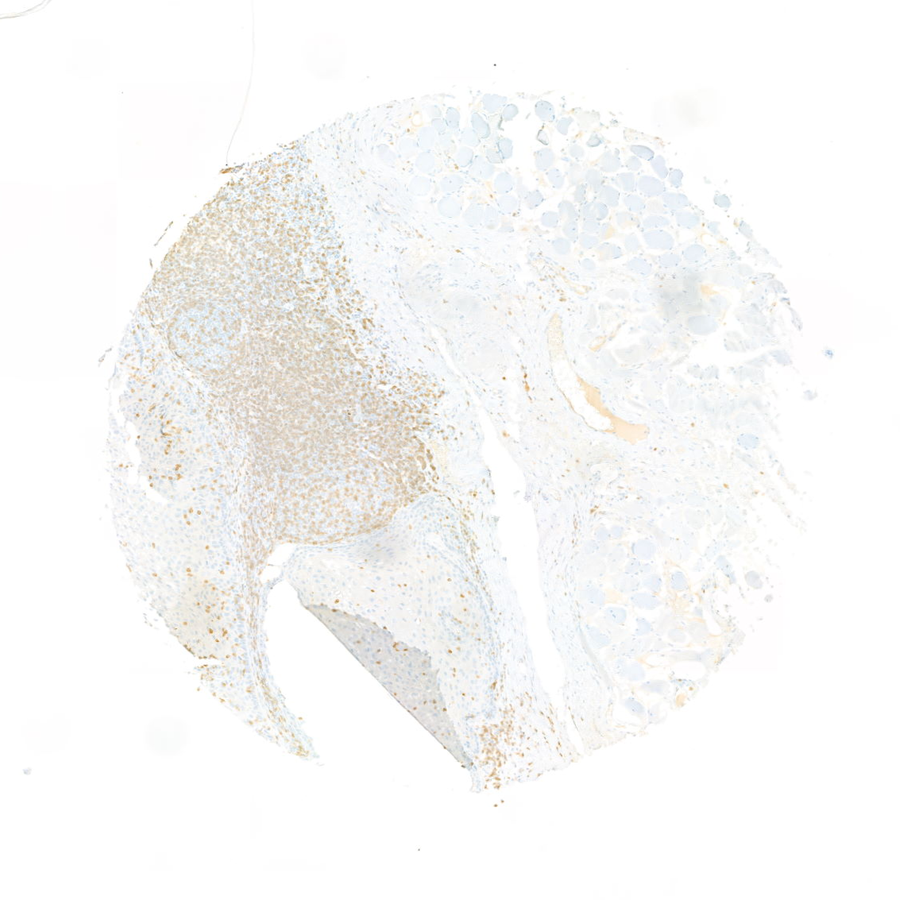}
\includegraphics[width=0.25\linewidth]{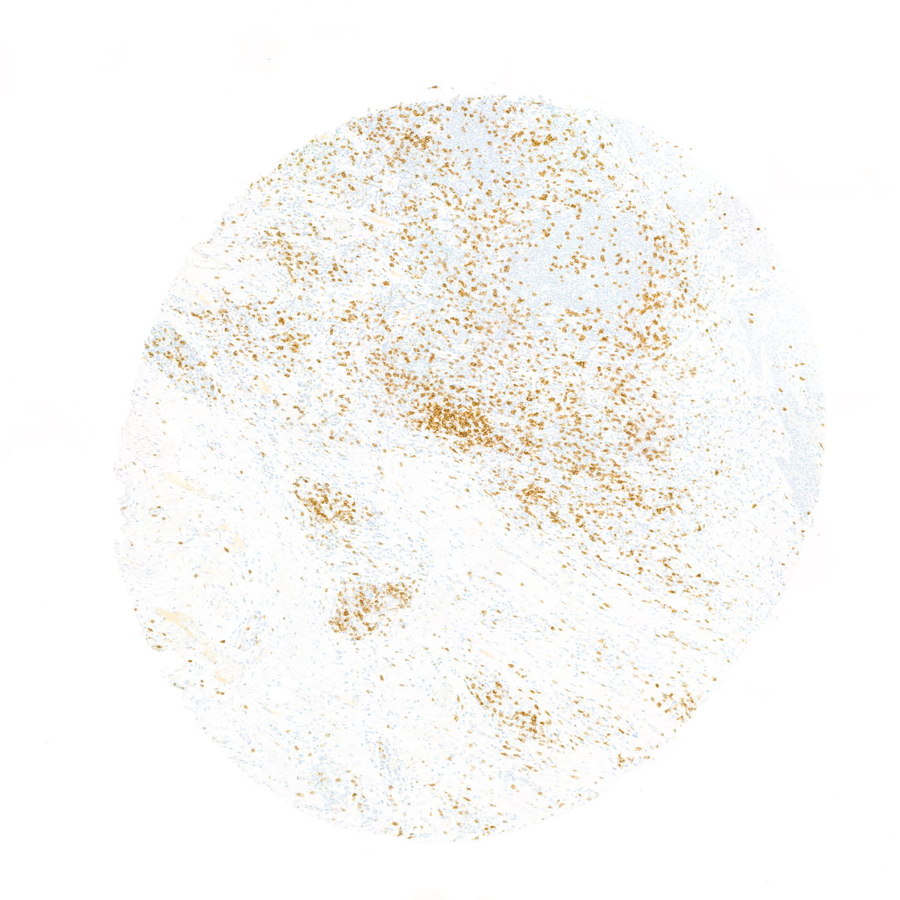}
\includegraphics[width=0.25\linewidth]{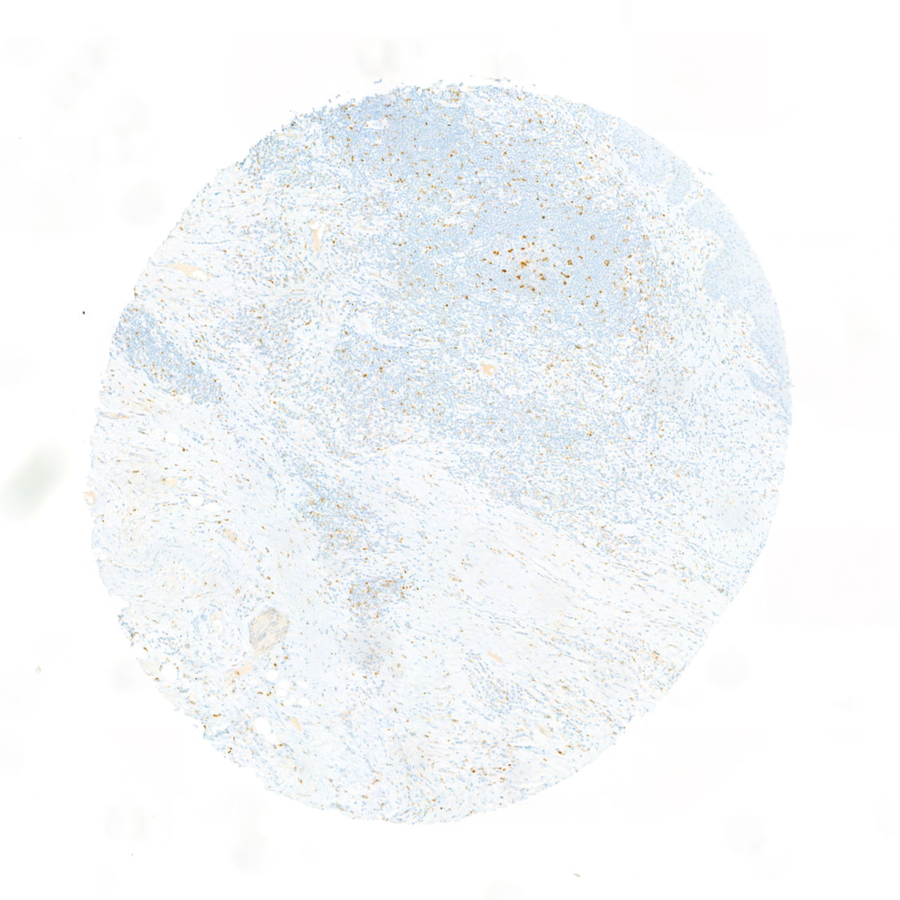}
\\
\textit{+ 6 other files}
\end{center}


    \textbf{Tools Used:} None
    \end{tcolorbox}
    \end{minipage}\hfill
    \begin{minipage}[t]{0.48\textwidth}
    \begin{tcolorbox}[title=Tools Available, colback=green!5, boxsep=1pt, left=2pt, right=2pt, top=2pt, bottom=2pt]
    \begin{tcolorbox}[colback=gray!10, title=Conversation, boxsep=1pt, left=1pt, right=1pt, top=1pt, bottom=1pt]
\textbf{User:} [IHCTool] + \textit{Question}\\
\textbf{Assistant:} To address the relationship between the observed perinodal invasion and immune cell infiltration at the InvasionFront, we need to consider the provided IHC data for various immune cell markers. Here is a summary of the relevant data:

- **CD3+ T-cell infiltration**: The TumorCenter has a higher CD3+ T-cell density compared to the InvasionFront.
- **CD8+ T-cell infiltration**: CD8+ T-cell infiltration is approximately equal in both regions.
- **CD56+ lymphocyte presence**: CD56+ lymphocytes are more abundant in the TumorCenter compared to the InvasionFront.
- **CD68+ macrophage infiltration**: The data provided does not specifically address CD68+ macrophage infiltration, so this cannot be directly evaluated.
- **PDL1 expression**: High PDL1 expression at the InvasionFront may contribute to immune evasion and facilitate metastasis.

Given the data, let's evaluate the options:

A) **High CD3+ and CD8+ T-cell infiltration likely prevents perinodal invasion**: The CD3+ T-cell infiltration is higher in the TumorCenter, but not significantly high in the InvasionFront. CD8+ T-cell infiltration is approximately equal in both regions. This does not strongly suggest prevention of perinodal invasion.

B) **High CD68+ macrophage infiltration at the InvasionFront may facilitate perinodal invasion**: There is no specific data provided on CD68+ macrophage infiltration, so this cannot be directly evaluated.

[...]
%C) **Low CD56+ lymphocyte presence at the InvasionFront**: CD56+ lymphocytes are more abundant in the TumorCenter compared to the InvasionFront. However, their presence does not directly indicate a lack of immune contribution to perinodal invasion.

D) **High PDL1 expression at the InvasionFront may contribute to immune evasion and perinodal invasion**: High PDL1 expression at the InvasionFront can contribute to immune evasion by inhibiting T-cell activity, which may facilitate perinodal invasion.

Given the high PDL1 expression at the InvasionFront, it is likely that this contributes to immune evasion and facilitates perinodal invasion. \\[1pt]
\end{tcolorbox}

    \textbf{Answer:} D) High PDL1 expression at the InvasionFront may contribute to immune evasion and perinodal invasion

    \textbf{Files Accessed:} 12 IHC images (same as left panel)\\
    \begin{center}
\end{center}
\textit{}


    \textbf{Tools Used:} IHC Tool
    \end{tcolorbox}
    \end{minipage}
    \end{tcolorbox}
